# Supplementary material for: Crossover from adiabatic to antiadiabatic quantum pumping with dissipation
Source: arXiv:1104.0815 source file (2011-08-30)
Supplement: Supplementary file 2 [file DD3SS_Suppl.pdf]

# Crossover from adiabatic to antiadiabatic quantum pumping with dissipation – Supplementary Material

Franco Pellegrini, C. Negri, F. Pistolesi, Nicola Manini, Giuseppe E. Santoro, and Erio Tosatti

In this supplementary material, we provide the explicit algebra relating two different realistic systems to the spin-1/2 Hamiltonian (1) studied in the paper: a triple quantum dot and a molecular trimer.

We also include a few details of the derivation of the explicit form of master equation for the spin in contact with a thermostat.

## Appendix A: Triple Quantum Dot

Consider a ring composed of three equal quantum dots [1]. Indicate with  $\epsilon_i$  the external bias applied to a single-orbital dot  $i$ , and  $\gamma_{ij}$  the hopping amplitude for an electron to jump between sites  $i$  and  $j$ . The Hamiltonian

$$\mathcal{H}_0 = \begin{pmatrix} \epsilon_a & -\gamma_{ab} & -\gamma_{ac} \\ -\gamma_{ab} & \epsilon_b & -\gamma_{bc} \\ -\gamma_{ac} & -\gamma_{bc} & \epsilon_c \end{pmatrix} \quad (\text{A1})$$

describes the one-electron dynamics. Without loss of generality, we measure energy in a scale such that  $\sum_i \epsilon_i = 0$ .

This Hamiltonian can be easily diagonalized in the fully symmetric case of equal hoppings  $\gamma_{ij} = \gamma_0$  and energies  $\epsilon_a = \epsilon_b = \epsilon_c = 0$ , to give a ground state  $|0\rangle = (|a\rangle + |b\rangle + |c\rangle)/\sqrt{3}$  with energy  $-2\gamma_0$  and a degenerate doublet of excited levels with energy  $\gamma_0$ . We choose as a basis for the degenerate subspace  $|x\rangle = (|b\rangle - |c\rangle)/\sqrt{2}$  and  $|y\rangle = (2|a\rangle - |b\rangle - |c\rangle)/\sqrt{6}$ . Neglecting electron-electron correlation effects, when three electrons occupy the system of the three quantum dots, two of them fill state  $|0\rangle$ , and the third one remains free to move in the twofold-degenerate manifold, which is therefore the one relevant for transport processes.

To act on this twofold degeneracy, experimentally the easiest way is to perturb the bias  $\epsilon_i$  at each site. One can consider the perturbing Hamiltonian in the  $|0\rangle$ ,  $|x\rangle$ ,  $|y\rangle$  basis:

$$\mathcal{H}_{\text{bias}} = \begin{pmatrix} 0 & \frac{1}{\sqrt{6}}(\epsilon_b - \epsilon_c) & \frac{1}{\sqrt{2}}\epsilon_a \\ \frac{1}{\sqrt{6}}(\epsilon_b - \epsilon_c) & -\frac{1}{2}\epsilon_a & \frac{1}{2\sqrt{3}}(\epsilon_c - \epsilon_b) \\ \frac{1}{\sqrt{2}}\epsilon_a & \frac{1}{2\sqrt{3}}(\epsilon_c - \epsilon_b) & \frac{1}{2}\epsilon_a \end{pmatrix}. \quad (\text{A2})$$

As long as the deviation from the unbiased system can be treated as a small perturbation with respect to the gap  $3\gamma_0$ , admixtures of state  $|0\rangle$  produce negligible effects within the  $|x\rangle$   $|y\rangle$  doublet. One can therefore restrict the treatment to the  $|x\rangle$   $|y\rangle$  subspace. Here, the perturbing Hamiltonian takes the form:

$$\mathcal{H}_{\text{QD}} = -\frac{1}{2\sqrt{3}} \begin{pmatrix} \sqrt{3}\epsilon_a & \epsilon_b - \epsilon_c \\ \epsilon_b - \epsilon_c & -\sqrt{3}\epsilon_a \end{pmatrix}. \quad (\text{A3})$$

By cycling the external potentials according to  $\epsilon_a = -\hbar\Delta \cos \omega t$ ,  $\epsilon_b = -\hbar\Delta \cos(\omega t - \frac{2\pi}{3})$ ,  $\epsilon_c = -\hbar\Delta \cos(\omega t + \frac{2\pi}{3})$  we reduce the system exactly to the spin-1/2 Hamiltonian, Eq. (1), which is the starting point the paper.

## Appendix B: Molecular Trimer

A different mechanism leading to the same Hamiltonian describes the electronic states of a molecular trimer such as in the molecules  $\text{H}_3$ ,  $\text{Li}_3$  or  $\text{Na}_3$  [2–5]. In such a system, the quantum dots are replaced by the valence electronic orbitals in a molecule. Driving is achieved through the excitation of “rotating” vibrational modes and acts through the degenerate electron-vibration interaction, of the Jahn-Teller “ $e \otimes E$ ” type [6–8]. Indeed, among the initial motivations for our study was the question whether the spontaneous chiral phonons generated during forced sliding of coaxial nanotubes [9] could act as a pump of chiral currents in the outer tube. However, while in that case too the pumping of a circular current would seem inescapable, the physics of the nanotube is far more complicated than the present model, and the question must await future work.

A standard tight-binding model [10] provides a basic and fairly realistic picture of the molecular electronic structure. For the case of a molecular trimer, the relevant tight-binding Hamiltonian reads exactly like Eq. (A1). A trimer of equal atoms has identical on-site energy  $\epsilon_a = \epsilon_b = \epsilon_c = 0$ . Here, what can change in time are the hopping integrals  $\gamma_{ij}$ . The equilateral molecular geometry has identical hopping integrals  $\gamma_{ij} = \gamma_0$ . In these conditions the spectrum consists again of a singlet ground state at energy  $-2\gamma_0$  plus a twofold degenerate excited state at energy  $\gamma_0$ .

Upon molecular distortion, these overlaps may be assumed to change with distance approximately as

$$\gamma_{ij} \simeq \gamma_0 e^{-\kappa(d_{ij} - u_0)}, \quad (\text{B1})$$

where  $d_{ij}$  is the instantaneous distance between atoms  $i$  and  $j$ , and  $u_0$  is the equilibrium separation in the equilateral geometry. Consider the perturbation to the electronic levels induced by the a small-amplitude excitation of the vibrational modes of the trimer. Excluding the uniform dilation, which does not split the degeneracy, the remaining two vibrational normal modes are degenerate in frequency. The associated atomic displaced positions can be described in terms of two normal coordinates  $Q_x$

and  $Q_y$  as follows:

$$\begin{cases} \mathbf{R}_a = (0, 1) \frac{u_0}{\sqrt{3}} + \left(\frac{1}{\sqrt{3}}, 0\right) Q_x + \left(0, \frac{1}{\sqrt{3}}\right) Q_y \\ \mathbf{R}_b = -\left(\frac{\sqrt{3}}{2}, \frac{1}{2}\right) \frac{u_0}{\sqrt{3}} - \left(\frac{1}{2\sqrt{3}}, \frac{1}{2}\right) Q_x + \left(\frac{1}{2}, \frac{-1}{2\sqrt{3}}\right) Q_y \\ \mathbf{R}_c = \left(\frac{\sqrt{3}}{2}, -\frac{1}{2}\right) \frac{u_0}{\sqrt{3}} + \left(\frac{-1}{2\sqrt{3}}, \frac{1}{2}\right) Q_x - \left(\frac{1}{2}, \frac{1}{2\sqrt{3}}\right) Q_y \end{cases} \quad (\text{B2})$$

The modified atomic positions result in modified overlap integrals estimated by substituting  $d_{ij} = |\mathbf{R}_i - \mathbf{R}_j|$  into Eq. (B1). We computed the electron-phonon linear coupling by linearizing the coupling term for small  $Q_i$ . We obtain the following overlaps

$$\begin{cases} \gamma_{ab} \simeq \gamma_0 \left(1 - \kappa \frac{\sqrt{3}}{2} Q_x - \kappa \frac{1}{2} Q_y\right) \\ \gamma_{bc} \simeq \gamma_0 \left(1 + \kappa Q_y\right) \\ \gamma_{ac} \simeq \gamma_0 \left(1 + \kappa \frac{\sqrt{3}}{2} Q_x - \kappa \frac{1}{2} Q_y\right) \end{cases} \quad (\text{B3})$$

The resulting Hamiltonian for perturbatively small displacement can be represented in the  $|0\rangle$ ,  $|x\rangle$ ,  $|y\rangle$  basis:

$$\mathcal{H}_{\text{lin}} = \gamma_0 \begin{pmatrix} -2 & \frac{1}{\sqrt{2}} \kappa Q_x & \frac{1}{\sqrt{2}} \kappa Q_y \\ \frac{1}{\sqrt{2}} \kappa Q_x & 1 + \kappa Q_y & \kappa Q_x \\ \frac{1}{\sqrt{2}} \kappa Q_y & \kappa Q_x & 1 - \kappa Q_y \end{pmatrix}. \quad (\text{B4})$$

We can further restrict this linearized Hamiltonian to the  $|x\rangle$ ,  $|y\rangle$  subspace, where it takes the form:

$$\mathcal{H}_{\text{MT}} = \kappa \gamma_0 \begin{pmatrix} Q_y & Q_x \\ Q_x & -Q_y \end{pmatrix}, \quad (\text{B5})$$

with the omission of the trivial shift by  $\gamma_0$ .

Assume that it is possible to excite a classical motion of the vibrational degree of freedom, and choose a time-dependent rotating combination of these vibrations with amplitudes  $Q_x = \frac{\hbar \Delta}{2\kappa \gamma_0} \sin(\omega t)$ ,  $Q_y = \frac{\hbar \Delta}{2\kappa \gamma_0} \cos(\omega t)$ . By plugging this dependency into Eq. (B5), the form (1) is once more recovered.

### Appendix C: The master equation for the density matrix

The master equation (5) can be written out explicitly in its simplest form in the rotating frame of reference where (2) is diagonal. We indicate the three orthonormal basic directions by  $\hat{\mathbf{x}} = (1, 0, 0)$ ,  $\hat{\mathbf{m}} = (0, \Delta/\omega', \omega/\omega')$ , and  $\hat{\mathbf{n}} = (0, -\omega/\omega', \Delta/\omega')$ . These axis are uniformly rotating at angular speed  $\omega$ , as dictated by the  $R_y(\omega t)$  transformation, relative to the inertial frame where the original spin problem Eq. (1) is formulated. Consider:

$$\begin{cases} \sigma^x = \hat{\mathbf{x}} \cdot \boldsymbol{\sigma} \\ \sigma^m = \hat{\mathbf{m}} \cdot \boldsymbol{\sigma} \\ \sigma^n = \hat{\mathbf{n}} \cdot \boldsymbol{\sigma}, \end{cases} \quad (\text{C1})$$

for which standard commutation relations hold, due to orthonormality. In terms of these operators we can rewrite the master equation (5) as

$$\begin{aligned} \frac{\partial \tilde{\rho}_S(t)}{\partial t} = & -i \frac{\omega'}{2} [\sigma^n, \tilde{\rho}_S] - \left[ \cos(\omega t) \sigma^x + \sin(\omega t) \left( \frac{\Delta}{\omega'} \sigma^n + \frac{\omega}{\omega'} \sigma^m \right), \right. \\ & \left\{ \frac{\Delta}{\omega'} (\sin(\omega t) g_{c0} + \cos(\omega t) g_{s0}) \sigma^n + \right. \\ & + \left( \cos(\omega t) g_{cc} - \sin(\omega t) g_{sc} + \frac{\omega}{\omega'} \sin(\omega t) g_{cs} \frac{\omega}{\omega'} \cos(\omega t) g_{ss} \right) \sigma^x + \\ & + \left. \left( \sin(\omega t) g_{ss} - \cos(\omega t) g_{cs} + \frac{\omega}{\omega'} \sin(\omega t) g_{cc} + \frac{\omega}{\omega'} \cos(\omega t) g_{sc} \right) \sigma^m \right\} \tilde{\rho}_S \Big] + \text{c.c.} + \\ & + \left[ -\sin(\omega t) \sigma^x + \cos(\omega t) \left( \frac{\Delta}{\omega'} \sigma^n + \frac{\omega}{\omega'} \sigma^m \right), \left\{ \frac{\Delta}{\omega'} (\cos(\omega t) g_{c0} + \sin(\omega t) g_{s0}) \sigma^n + \right. \right. \\ & + \left( -\sin(\omega t) g_{cc} - \cos(\omega t) g_{sc} + \frac{\omega}{\omega'} \cos(\omega t) g_{cs} - \frac{\omega}{\omega'} \sin(\omega t) g_{ss} \right) \sigma^x + \\ & + \left. \left( \sin(\omega t) g_{cs} + \cos(\omega t) g_{ss} + \frac{\omega}{\omega'} \cos(\omega t) g_{cc} - \frac{\omega}{\omega'} \sin(\omega t) g_{sc} \right) \sigma^m \right\} \tilde{\rho}_S \Big] + \text{c.c.} \end{aligned} \quad (\text{C2})$$

We evaluate all commutators and reduce Eq. (C2) to a form where all coefficients of the density matrix at the right-hand side are constant in time. If we parameterize the density matrix as  $\tilde{\rho}_S(t) = \frac{1}{2} (\mathbb{I} + a(t) \sigma^x + b(t) \sigma^m + c(t) \sigma^n)$ ,

the master equation (C2) can be written

$$\begin{aligned}
\frac{\partial \tilde{\rho}_S(t)}{\partial t} = & -2 \left\{ \left( \frac{\Delta^2}{\omega'^2} \Re g_{c0} + \frac{\omega}{\omega'} \Re g_{ss} + \frac{\omega^2}{\omega'^2} \Re g_{cc} \right) a + \left( \frac{\omega'}{4} + \frac{\omega}{\omega'} \Re g_{sc} - \frac{\omega^2}{\omega'^2} \Re g_{cs} \right) b + \right. \\
& + \frac{\Delta}{\omega'} \left( \Re g_{sc} - \frac{\omega}{\omega'} \Re g_{cs} \right) c + \frac{\Delta}{\omega'} \left( -\frac{\omega}{\omega'} \Im g_{c0} + \Im g_{ss} + \frac{\omega}{\omega'} \Im g_{cc} \right) \left. \right\} \sigma^x + \\
& -2 \left\{ \left( -\frac{\omega'}{4} - \frac{\omega}{\omega'} \Re g_{sc} + \Re g_{cs} \right) a + \left( \frac{\Delta^2}{\omega'^2} \Re g_{c0} + \Re g_{cc} + \frac{\omega}{\omega'} \Re g_{ss} \right) b + \right. \\
& - \frac{\Delta}{\omega'} \left( \frac{\omega}{\omega'} \Re g_{cc} + \Re g_{ss} \right) c + \frac{\Delta}{\omega'} \left( \Im g_{s0} + \Im g_{sc} - \frac{\omega}{\omega'} \Im g_{cs} \right) \left. \right\} \sigma^m + \\
& -2 \left\{ -\frac{\Delta}{\omega'} \Re g_{s0} a - \frac{\omega}{\omega'} \frac{\Delta}{\omega'} \Re g_{c0} b + \left( \frac{\omega^2 + \omega'^2}{\omega'^2} \Re g_{cc} + 2 \frac{\omega}{\omega'} \Re g_{ss} \right) c + \left( -2 \frac{\omega}{\omega'} \Im g_{sc} + \frac{\omega^2 + \omega'^2}{\omega'^2} \Im g_{cs} \right) \right\} \sigma^n.
\end{aligned} \tag{C3}$$

The constant coefficients in the above expression involve the following integrals of the environment correlation functions  $G_x(\tau) = G_z(\tau) \equiv G(\tau)$ :

$$g_{cc} = \int_0^\infty G(\tau) \cos(-\omega\tau) \cos(-\omega'\tau) d\tau \tag{C4}$$

$$g_{sc} = \int_0^\infty G(\tau) \sin(-\omega\tau) \cos(-\omega'\tau) d\tau \tag{C5}$$

$$g_{cs} = \int_0^\infty G(\tau) \cos(-\omega\tau) \sin(-\omega'\tau) d\tau \tag{C6}$$

$$g_{ss} = \int_0^\infty G(\tau) \sin(-\omega\tau) \sin(-\omega'\tau) d\tau \tag{C7}$$

$$g_{c0} = \int_0^\infty G(\tau) \cos(-\omega\tau) d\tau \tag{C8}$$

$$g_{s0} = \int_0^\infty G(\tau) \sin(-\omega\tau) d\tau. \tag{C9}$$

The coefficients  $a(t)$  and  $b(t)$ , appearing in the off-diagonal elements of the density matrix in the adopted representation, can be shown to approach zero. The coefficient  $c(t)$ , appearing in the diagonal elements (the statistical “population” of states), is related to the polarization discussed in the paper by  $P = -\text{Tr}(\hat{\mathbf{n}} \cdot \boldsymbol{\sigma} \tilde{\rho}_S) = -c$ . Inspection of the last line of Eq. (C3), setting to zero at stationarity the coefficient of the  $\sigma^n$  term, leads to the exact expression for the polarization, Eq. (6), given in the paper.

- 
- [1] L. Gaudreau, S. A. Studenikin, A. S. Sachrajda, P. Zawadzki, A. Kam, J. Lapointe, M. Korkusinski, and P. Hawrylak, Phys. Rev. Lett. **97**, 036807 (2006).
  - [2] W. H. Gerber, and E. Schumacher, J. Chem. Phys. **69**, 1692 (1978).
  - [3] G. Delacrétaz, E. R. Grant, R. L. Whetten, L. Wöste, and J. W. Zwanziger, Phys. Rev. Lett. **56**, 2598 (1986).
  - [4] Ph. Dugourd, J. Chevalere, J. P. Perrot, and M. Broyer, J. Chem. Phys. **93**, 2332 (1990).
  - [5] P. Dugourd, J. Chevalere, R. Antoine, M. Broyer, J. P. Wolf, and L. Wöste, Chem. Phys. Lett. **225**, 28 (1994).
  - [6] R. Englman, *The Jahn Teller Effect in Molecules and*

- Crystals* (Wiley, London, 1972).
- [7] I. B. Bersuker and V. Z. Polinger, *Vibronic Interactions in Molecules and Crystals* (Springer-Verlag, Berlin, 1989).
- [8] I. B. Bersuker, *The Jahn-Teller effect* (Cambridge Univ. Press, Cambridge, 2006).
- [9] X. H. Zhang, Giuseppe E. Santoro, U. Tartaglino, E. Tosatti, Phys. Rev. Lett. **102**, 125502 (2009).
- [10] N. W. Ashcroft and M. D. Mermin, *Solid State Physics* (Holt-Saunders, Philadelphia, 1976).
